# Supplementary material for: LiDAR-based 4D Panoptic Segmentation via Dynamic Shifting Network
Source: arXiv:2203.07186 source file (2022-03-14)
Supplement: Supplementary file 1 [file supp_colab.tex]

\begin{figure*}[t]
    \begin{center}
        \includegraphics[width=1.0\linewidth]{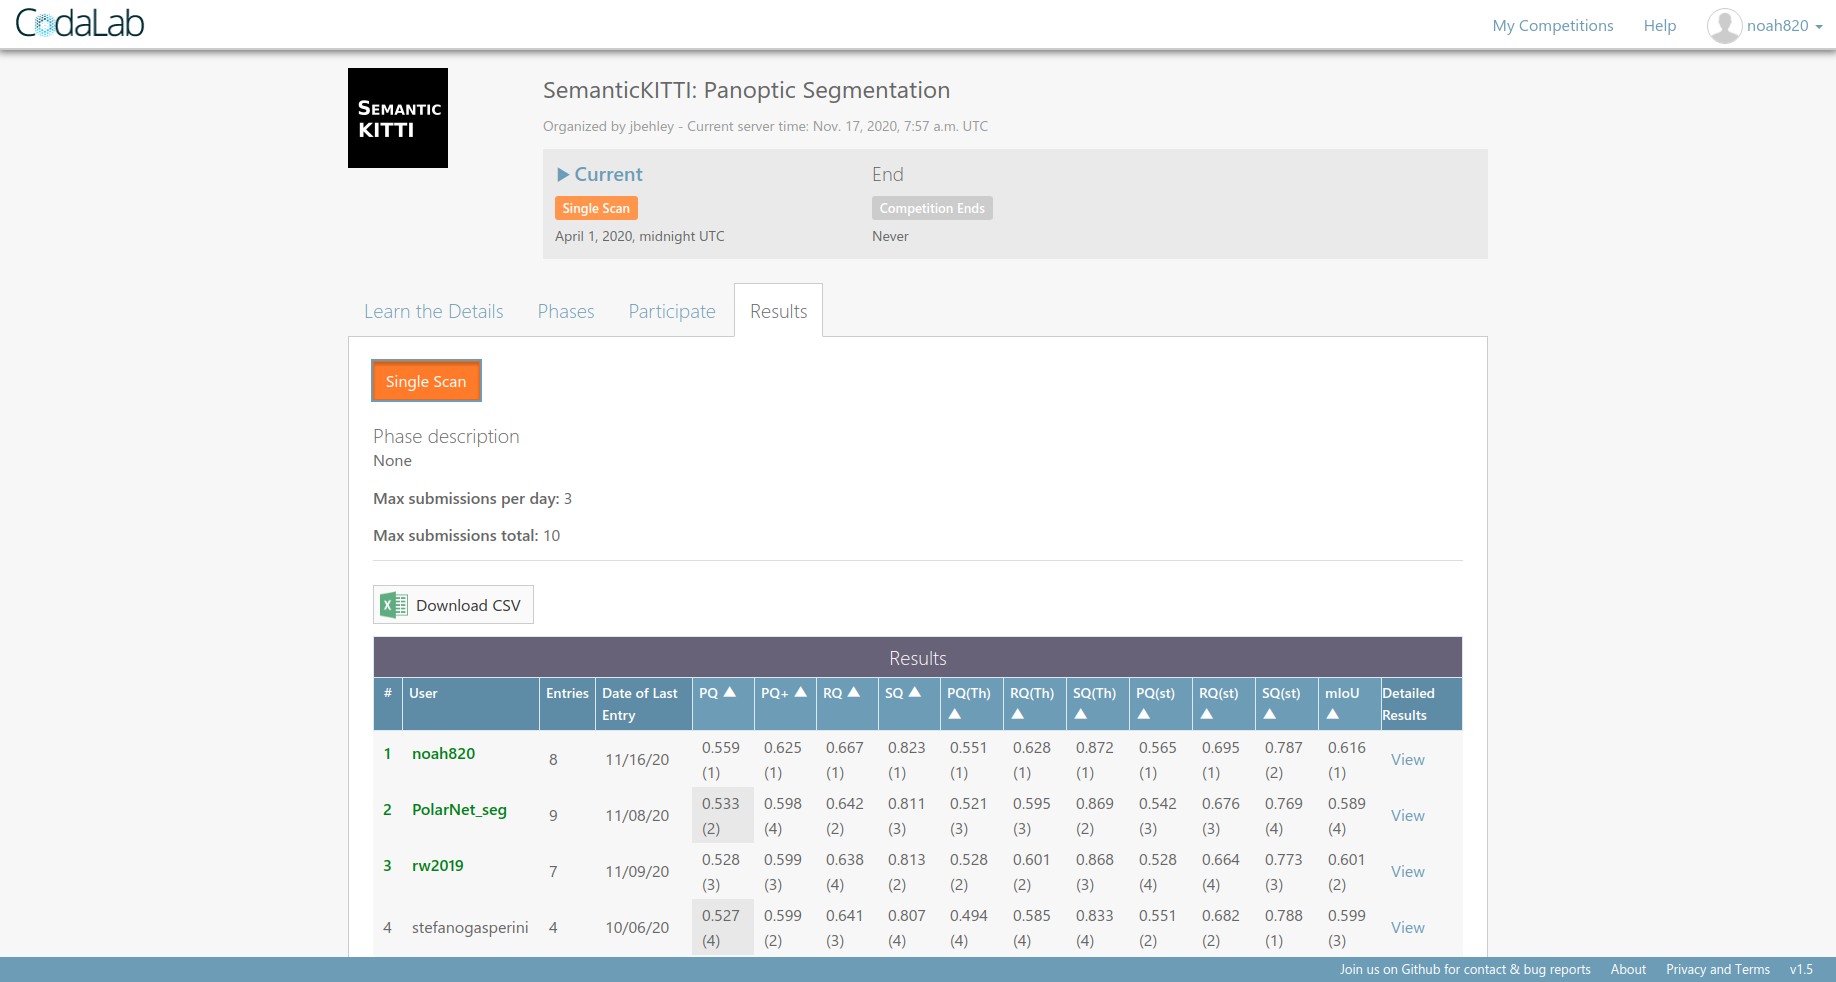}
    \end{center}
    \caption{Screenshot of the public leaderboard (\url{https://competitions.codalab.org/competitions/24025}) of SemanticKITTI at 2020-11-16. Our method achieves 1st place.}
    \label{fig:supp_colab}
\end{figure*}
